# Supplementary material for: Algorithmic Randomness and Kolmogorov Complexity for Qubits
Source: arXiv:2106.14280 source file (2021-06-27)
Supplement: Supplementary file 1 [file appendix.tex]

\chapter{Classical identities}\label{appendix}
%\fixchapterheading
